# Supplementary material for: Adversarial Stein Training for Graph Energy Models
Source: arXiv:2108.12982 source file (2021-08-30)
Supplement: Supplementary file 1 [file appendix2.tex]

\allowdisplaybreaks
\appendix

\onecolumn

\section{Architecture}
\label{app:edp}
\tikzset{every picture/.style={line width=0.75pt}} %set default line width to 0.75pt        

\begin{figure}
\centering
\begin{tikzpicture}[x=0.75pt,y=0.75pt,yscale=-1,xscale=1]
%uncomment if require: \path (0,300); %set diagram left start at 0, and has height of 300

%Rounded Rect [id:dp5705790113865654] 
\draw   (53,49) .. controls (53,44.58) and (56.58,41) .. (61,41) -- (115,41) .. controls (119.42,41) and (123,44.58) .. (123,49) -- (123,73) .. controls (123,77.42) and (119.42,81) .. (115,81) -- (61,81) .. controls (56.58,81) and (53,77.42) .. (53,73) -- cycle ;
%Rounded Rect [id:dp17838882825977742] 
\draw   (55,157.2) .. controls (55,154.33) and (57.33,152) .. (60.2,152) -- (102.3,152) .. controls (105.17,152) and (107.5,154.33) .. (107.5,157.2) -- (107.5,172.8) .. controls (107.5,175.67) and (105.17,178) .. (102.3,178) -- (60.2,178) .. controls (57.33,178) and (55,175.67) .. (55,172.8) -- cycle ;
%Rounded Rect [id:dp9034731403411416] 
\draw   (175,49) .. controls (175,44.58) and (178.58,41) .. (183,41) -- (237,41) .. controls (241.42,41) and (245,44.58) .. (245,49) -- (245,73) .. controls (245,77.42) and (241.42,81) .. (237,81) -- (183,81) .. controls (178.58,81) and (175,77.42) .. (175,73) -- cycle ;
%Rounded Rect [id:dp6527588946958224] 
\draw   (184,158.2) .. controls (184,155.33) and (186.33,153) .. (189.2,153) -- (231.3,153) .. controls (234.17,153) and (236.5,155.33) .. (236.5,158.2) -- (236.5,173.8) .. controls (236.5,176.67) and (234.17,179) .. (231.3,179) -- (189.2,179) .. controls (186.33,179) and (184,176.67) .. (184,173.8) -- cycle ;
%Flowchart: Merge [id:dp8068060170933739] 
\draw   (175,100) -- (245,100) -- (210,140) -- cycle ;
%Shape: Triangle [id:dp9050789006095706] 
\draw   (353.75,60.35) -- (290.5,79) -- (290.5,42) -- cycle ;
%Rounded Rect [id:dp5135714413276413] 
\draw   (376,48) .. controls (376,43.58) and (379.58,40) .. (384,40) -- (438,40) .. controls (442.42,40) and (446,43.58) .. (446,48) -- (446,72) .. controls (446,76.42) and (442.42,80) .. (438,80) -- (384,80) .. controls (379.58,80) and (376,76.42) .. (376,72) -- cycle ;
%Flowchart: Merge [id:dp21729120393106038] 
\draw   (381,102) -- (451,102) -- (416,142) -- cycle ;
%Rounded Rect [id:dp32285537820930277] 
\draw   (392,158.2) .. controls (392,155.33) and (394.33,153) .. (397.2,153) -- (439.3,153) .. controls (442.17,153) and (444.5,155.33) .. (444.5,158.2) -- (444.5,173.8) .. controls (444.5,176.67) and (442.17,179) .. (439.3,179) -- (397.2,179) .. controls (394.33,179) and (392,176.67) .. (392,173.8) -- cycle ;
%Shape: Triangle [id:dp727699880788818] 
\draw   (544.75,59.36) -- (481.5,77) -- (481.5,42) -- cycle ;
%Rounded Rect [id:dp07969997725904854] 
\draw   (564,50) .. controls (564,45.58) and (567.58,42) .. (572,42) -- (626,42) .. controls (630.42,42) and (634,45.58) .. (634,50) -- (634,74) .. controls (634,78.42) and (630.42,82) .. (626,82) -- (572,82) .. controls (567.58,82) and (564,78.42) .. (564,74) -- cycle ;
%Straight Lines [id:da21931788822628207] 
\draw  [dash pattern={on 0.84pt off 2.51pt}]  (124.5,62) -- (174.5,62) ;
\draw [shift={(176.5,62)}, rotate = 180] [color={rgb, 255:red, 0; green, 0; blue, 0 }  ][line width=0.75]    (10.93,-3.29) .. controls (6.95,-1.4) and (3.31,-0.3) .. (0,0) .. controls (3.31,0.3) and (6.95,1.4) .. (10.93,3.29)   ;
%Straight Lines [id:da7674968898261304] 
\draw  [dash pattern={on 0.84pt off 2.51pt}]  (86.5,85) -- (86.5,150) ;
\draw [shift={(86.5,152)}, rotate = 270] [color={rgb, 255:red, 0; green, 0; blue, 0 }  ][line width=0.75]    (10.93,-3.29) .. controls (6.95,-1.4) and (3.31,-0.3) .. (0,0) .. controls (3.31,0.3) and (6.95,1.4) .. (10.93,3.29)   ;
%Straight Lines [id:da5281865002961916] 
\draw    (207.5,84) -- (207.5,101) ;
%Curve Lines [id:da2144906514859819] 
\draw    (110.5,165) .. controls (199.5,168) and (98.5,87) .. (208.5,91) ;
%Curve Lines [id:da959149478498903] 
\draw    (239.5,167) .. controls (389.5,167) and (233.5,92) .. (411.5,95) ;
%Curve Lines [id:da3001738199865235] 
\draw    (447.5,168) .. controls (493.5,171) and (449.5,61) .. (481.5,59) ;
%Straight Lines [id:da32612247406171313] 
\draw    (210,140) -- (210.5,152) ;
%Straight Lines [id:da36283245761216676] 
\draw    (411.5,82) -- (411.5,101) ;
%Straight Lines [id:da9445959292762895] 
\draw    (416,142) -- (415.5,152) ;
%Straight Lines [id:da8961301679878532] 
\draw    (246.5,61) -- (288.5,61) ;
%Straight Lines [id:da7375375765678399] 
\draw    (262.5,63) -- (263,168) ;
%Straight Lines [id:da3449445003165621] 
\draw    (353.75,60.35) -- (376.5,60) ;
%Straight Lines [id:da8477700294725956] 
\draw    (448.5,59) -- (481.5,59) ;
%Straight Lines [id:da6072965229542594] 
\draw    (207.5,40) -- (207.5,15) ;
%Straight Lines [id:da5856155358442884] 
\draw    (207.5,15) -- (459.5,17) ;
%Straight Lines [id:da7326331867626164] 
\draw    (459.5,17) -- (481.5,59) ;
%Straight Lines [id:da9598306124311234] 
\draw    (544.75,59.36) -- (563.5,59) ;

% Text Node
\draw (66,53) node [anchor=north west][inner sep=0.75pt]   [align=left] { \ Adj: $ \bm{X} $};
% Text Node
\draw (62.2,155) node [anchor=north west][inner sep=0.75pt]   [align=left] { \ $ \bm{h}_0$ };
% Text Node
\draw (194,54) node [anchor=north west][inner sep=0.75pt]   [align=left] {\textbf{ $\bm{A}_0$ }};
% Text Node
\draw (192.2,106) node [anchor=north west][inner sep=0.75pt]   [align=left] {GNN};
% Text Node
\draw (191.2,156) node [anchor=north west][inner sep=0.75pt]   [align=left] {\textbf{ \ $\bm{h}_1$}};
% Text Node
\draw (292.2,53) node [anchor=north west][inner sep=0.75pt]   [align=left] {MLP};
% Text Node
\draw (484.2,51) node [anchor=north west][inner sep=0.75pt]   [align=left] {MLP};
% Text Node
\draw (398.2,107) node [anchor=north west][inner sep=0.75pt]   [align=left] {GNN};
% Text Node
\draw (395,52) node [anchor=north west][inner sep=0.75pt]   [align=left] {\textbf{ $\bm{A}_1$ }};
% Text Node
\draw (582,52) node [anchor=north west][inner sep=0.75pt]   [align=left] {\textbf{$\bm{E}_\theta$}};
% Text Node
\draw (399.2,156) node [anchor=north west][inner sep=0.75pt]   [align=left] {\textbf{ \ $\bm{h}_2$}};

\end{tikzpicture}
\caption{Example architecture of EDPGNN ~\citep{niu2020permutation}  \label{fig:edpgnn}}
\end{figure}

\begin{figure}
\centering

%\tikzset{every picture/.style={line width=0.75pt}} %set default line width to 0.75pt        
\begin{tikzpicture}[x=0.75pt,y=0.75pt,yscale=-1,xscale=1]
%uncomment if require: \path (0,300); %set diagram left start at 0, and has height of 300

%Shape: Rectangle [id:dp7777338471558682] 
%Shape: Rectangle [id:dp7777338471558682] 
\draw   (73.75,70) -- (195.25,70) -- (195.25,148) -- (73.75,148) -- cycle ;
%Flowchart: Connector [id:dp43909903365607006] 
\draw   (100,87) .. controls (100,83.69) and (103.92,81) .. (108.75,81) .. controls (113.58,81) and (117.5,83.69) .. (117.5,87) .. controls (117.5,90.31) and (113.58,93) .. (108.75,93) .. controls (103.92,93) and (100,90.31) .. (100,87) -- cycle ;
%Flowchart: Connector [id:dp8725228978373948] 
\draw   (144,90) .. controls (144,86.69) and (147.92,84) .. (152.75,84) .. controls (157.58,84) and (161.5,86.69) .. (161.5,90) .. controls (161.5,93.31) and (157.58,96) .. (152.75,96) .. controls (147.92,96) and (144,93.31) .. (144,90) -- cycle ;
%Flowchart: Connector [id:dp3266101845718349] 
\draw   (120.25,105) .. controls (120.25,101.69) and (124.17,99) .. (129,99) .. controls (133.83,99) and (137.75,101.69) .. (137.75,105) .. controls (137.75,108.31) and (133.83,111) .. (129,111) .. controls (124.17,111) and (120.25,108.31) .. (120.25,105) -- cycle ;
%Flowchart: Connector [id:dp7380863711127121] 
\draw   (147,127) .. controls (147,123.69) and (150.92,121) .. (155.75,121) .. controls (160.58,121) and (164.5,123.69) .. (164.5,127) .. controls (164.5,130.31) and (160.58,133) .. (155.75,133) .. controls (150.92,133) and (147,130.31) .. (147,127) -- cycle ;
%Flowchart: Connector [id:dp5826639776056545] 
\draw   (123,130) .. controls (123,126.69) and (126.92,124) .. (131.75,124) .. controls (136.58,124) and (140.5,126.69) .. (140.5,130) .. controls (140.5,133.31) and (136.58,136) .. (131.75,136) .. controls (126.92,136) and (123,133.31) .. (123,130) -- cycle ;
%Straight Lines [id:da24290367526914836] 
\draw    (108.75,93) -- (122.75,102) ;
%Straight Lines [id:da5889857944424571] 
\draw    (137.75,105) -- (152.75,96) ;
%Straight Lines [id:da710253880700211] 
\draw    (117.5,87) -- (144,90) ;
%Straight Lines [id:da9971350495767625] 
\draw    (129,111) -- (131.75,124) ;
%Straight Lines [id:da7282128112432816] 
\draw    (134.5,109) -- (149.5,122) ;
%Straight Lines [id:da7408384840783642] 
\draw    (204.5,102) -- (261.5,102) ;
\draw [shift={(263.5,102)}, rotate = 180] [color={rgb, 255:red, 0; green, 0; blue, 0 }  ][line width=0.75]    (10.93,-3.29) .. controls (6.95,-1.4) and (3.31,-0.3) .. (0,0) .. controls (3.31,0.3) and (6.95,1.4) .. (10.93,3.29)   ;
%Straight Lines [id:da10659821095511501] 
\draw    (306.5,102) -- (357.5,102) ;
\draw [shift={(359.5,102)}, rotate = 180] [color={rgb, 255:red, 0; green, 0; blue, 0 }  ][line width=0.75]    (10.93,-3.29) .. controls (6.95,-1.4) and (3.31,-0.3) .. (0,0) .. controls (3.31,0.3) and (6.95,1.4) .. (10.93,3.29)   ;
%Shape: Rectangle [id:dp0626356450381057] 
\draw   (366,86) -- (457.5,86) -- (457.5,126) -- (366,126) -- cycle ;
%Straight Lines [id:da3807478147059722] 
\draw    (469.5,101) -- (505.5,101) ;
\draw [shift={(507.5,101)}, rotate = 180] [color={rgb, 255:red, 0; green, 0; blue, 0 }  ][line width=0.75]    (10.93,-3.29) .. controls (6.95,-1.4) and (3.31,-0.3) .. (0,0) .. controls (3.31,0.3) and (6.95,1.4) .. (10.93,3.29)   ;
%Flowchart: Process [id:dp9227623574388255] 
\draw   (260,159) -- (336.5,159) -- (336.5,187) -- (260,187) -- cycle ;
%Shape: Rectangle [id:dp31229999666688035] 
\draw   (450.5,152) -- (487.5,152) -- (487.5,183) -- (450.5,183) -- cycle ;
%Curve Lines [id:da8825981286468081] 
\draw  [dash pattern={on 0.84pt off 2.51pt}]  (473.5,187) .. controls (477.48,242.72) and (339.89,251.91) .. (313.88,188.95) ;
\draw [shift={(313.5,188)}, rotate = 428.65999999999997] [color={rgb, 255:red, 0; green, 0; blue, 0 }  ][line width=0.75]    (10.93,-3.29) .. controls (6.95,-1.4) and (3.31,-0.3) .. (0,0) .. controls (3.31,0.3) and (6.95,1.4) .. (10.93,3.29)   ;
%Curve Lines [id:da10343443877295178] 
\draw  [dash pattern={on 0.84pt off 2.51pt}]  (488.5,168) .. controls (606.5,124) and (567.5,10) .. (438.5,86) ;
\draw [shift={(438.5,86)}, rotate = 329.5] [color={rgb, 255:red, 0; green, 0; blue, 0 }  ][line width=0.75]    (10.93,-3.29) .. controls (6.95,-1.4) and (3.31,-0.3) .. (0,0) .. controls (3.31,0.3) and (6.95,1.4) .. (10.93,3.29)   ;
%Straight Lines [id:da7762669034546712] 
\draw    (519.5,115) -- (489.67,156.38) ;
\draw [shift={(488.5,158)}, rotate = 305.79] [color={rgb, 255:red, 0; green, 0; blue, 0 }  ][line width=0.75]    (10.93,-3.29) .. controls (6.95,-1.4) and (3.31,-0.3) .. (0,0) .. controls (3.31,0.3) and (6.95,1.4) .. (10.93,3.29)   ;
%Straight Lines [id:da7679694481329302] 
\draw    (339.5,169) -- (377.5,169) ;
\draw [shift={(379.5,169)}, rotate = 180] [color={rgb, 255:red, 0; green, 0; blue, 0 }  ][line width=0.75]    (10.93,-3.29) .. controls (6.95,-1.4) and (3.31,-0.3) .. (0,0) .. controls (3.31,0.3) and (6.95,1.4) .. (10.93,3.29)   ;
%Straight Lines [id:da6361384361883543] 
\draw    (407.5,169) -- (445.5,169) ;
\draw [shift={(447.5,169)}, rotate = 180] [color={rgb, 255:red, 0; green, 0; blue, 0 }  ][line width=0.75]    (10.93,-3.29) .. controls (6.95,-1.4) and (3.31,-0.3) .. (0,0) .. controls (3.31,0.3) and (6.95,1.4) .. (10.93,3.29)   ;
%Straight Lines [id:da8075563669295907] 
\draw    (170.5,186) -- (211.9,155.19) ;
\draw [shift={(213.5,154)}, rotate = 503.34] [color={rgb, 255:red, 0; green, 0; blue, 0 }  ][line width=0.75]    (10.93,-3.29) .. controls (6.95,-1.4) and (3.31,-0.3) .. (0,0) .. controls (3.31,0.3) and (6.95,1.4) .. (10.93,3.29)   ;
%Shape: Rectangle [id:dp6554770674867495] 
\draw   (140.5,186) -- (168.5,186) -- (168.5,208) -- (140.5,208) -- cycle ;
%Straight Lines [id:da9639017656535334] 
\draw    (245.5,136) -- (270.09,111.41) ;
\draw [shift={(271.5,110)}, rotate = 495] [color={rgb, 255:red, 0; green, 0; blue, 0 }  ][line width=0.75]    (10.93,-3.29) .. controls (6.95,-1.4) and (3.31,-0.3) .. (0,0) .. controls (3.31,0.3) and (6.95,1.4) .. (10.93,3.29)   ;
%Straight Lines [id:da20247427974296217] 
\draw    (287.5,114) -- (293.72,158.02) ;
\draw [shift={(294,160)}, rotate = 261.96] [color={rgb, 255:red, 0; green, 0; blue, 0 }  ][line width=0.75]    (10.93,-3.29) .. controls (6.95,-1.4) and (3.31,-0.3) .. (0,0) .. controls (3.31,0.3) and (6.95,1.4) .. (10.93,3.29)   ;

% Text Node
\draw (180,93) node [anchor=north west][inner sep=0.75pt]   [align=left] {$\bm{A}$};
% Text Node
\draw (147,192) node [anchor=north west][inner sep=0.75pt]   [align=left] {$\sigma_i$};
% Text Node
\draw (274,93) node [anchor=north west][inner sep=0.75pt]   [align=left] {$\bm{A}_{\sigma_i}$};
% Text Node
\draw (379,97) node [anchor=north west][inner sep=0.75pt]   [align=left] {EDPGNN};
% Text Node
\draw (519,93) node [anchor=north west][inner sep=0.75pt]   [align=left] {$\bm{E}_\theta$};
% Text Node
\draw (264,164) node [anchor=north west][inner sep=0.75pt]   [align=left] {EDPGNN};
% Text Node
\draw (388,160) node [anchor=north west][inner sep=0.75pt]   [align=left] {$\bm{C}_\psi$};
% Text Node
\draw (463,158) node [anchor=north west][inner sep=0.75pt]   [align=left] {$\bm{S}$};
% Text Node
\draw (363,202) node [anchor=north west][inner sep=0.75pt]   [align=left] {Maximize};
% Text Node
\draw (557,75) node [anchor=north west][inner sep=0.75pt]   [align=left] {Minimize};
% Text Node
\draw (218,136) node [anchor=north west][inner sep=0.75pt]   [align=left] {$\mathcal{N}(0, \sigma_i^2)$};

\end{tikzpicture}

\caption{ \MODEL \space architecture  \label{fig:astra}}
\end{figure}

In Figure ~\ref{fig:astra} we pictorially represent the \MODEL \space architecture. Both the critic function $C$ and the energy $E$ are outputs of an EDPGNN architecture. One of the networks is trained to maximize the discrepancy $S$ while the other network minimizes $S$ in an adversarial game. The noise level $\sigma$ governs the corruptions to $A$ and provides robustness against critic overfitting. An example EDPGNN architecture is presented in Figure ~\ref{fig:edpgnn}. $h$ represent node and edge level feature representations. In an EDPGNN a multichannel GNN networks aggregates processed node and edge features in accordance to the matrix $A$ in one round of message passing. This layer can be stacked multiple times. The final output is obtained by aggregating $h$ and $A$ across all such stacked layers.

\section{Node Label Generation for Molecular Graphs}
In our initial experiments, we found that while our model can predict the graph structure quite accurately, the output of Langevin dynamics for the node labels (which in this case are the atom types) was comparatively poorer. As such to label the nodes for evaluating molecule validity we had to couple our model with the GraphAF model of \citet{shi2020graphaf}. The GraphAF model predicts the molecule autoregressively, which allows us to integrate it smoothly with our approach. Instead of relying however on GraphAF model to predict edges we simply present our edge predictions to the model. For node predictions we simply read off the node value as predicted by the GraphAF model.
